# Supplementary material for: SLM: Bridge the thin gap between speech and text foundation models
Source: arXiv:2310.00230 source file (2023-09-30)
Supplement: Supplementary file 1 [file appendix.tex]

\section{Appendix}
\label{sec:appendix}

\begin{table}[h]
\vspace{-.1in}
\centering
\rowcolors{6}{gray!25}{}
\begin{tabular}{ll}
\toprule
\textbf{Instruction} & \textbf{Prediction} \\
    \midrule
\midrule

\midrule
\multicolumn{2}{l}{\textbf{Audio Content} (From NQ dataset): When was the death penalty reinstated in oregon} \\
\hdashline

\hdashline
How do you answer this?  & 2002 / [\textcolor{red}{Groundtruth: 1984}] \\

\midrule
\multicolumn{2}{l}{\textbf{Audio Content} (From NQ dataset): How many wars held between india and pakistan} \\
\hdashline

\hdashline
How do you answer this?  & four wars, including one undeclared war / \\ & [\textcolor{red}{Groundtruth: There have been three wars between India and Pakistan.}] \\

\bottomrule
\end{tabular}
\caption{Failure cases of zero-shot instruction following on speech inputs.}
\label{0-shot_lemon}
% \vspace{-.1in}
\end{table}
